# Supplementary material for: Linear and nonlinear optical probe of the ferroelectric-like phase transition in a polar metal, LiOsO3
Source: arXiv:1809.05768 ancillary file (2018-09-15)
Supplement: Supplementary file 1 [file SM.pdf]

**Linear and nonlinear optical probe of the ferroelectric-like phase transition in a polar metal, $LiOsO_3$ - Supplementary Material**

Haricharan Padmanabhan,[1] Yoonsang Park,[1] Danilo Puggioni,[2] Yakun Yuan,[1] Yanwei Cao,[3] Lev Gasparov,[4] Youguo Shi,[5] Jak Chakhalian,[3] James M. Rondinelli,[2] and Venkatraman Gopalan[1, a)]

[1)] *Department of Materials Science and Engineering, The Pennsylvania State University, University Park, PA 16801, USA*

[2)] *Department of Materials Science and Engineering, Northwestern University, Evanston, IL 60208, USA*

[3)] *Department of Physics and Astronomy, Rutgers University, Piscataway, NJ 08854, USA*

[4)] *Department of Physics, University of North Florida, 1 UNF Drive Jacksonville, FL 32224, USA*

[5)] *Institute of Physics, Chinese Academy of Sciences, Beijing 100190, China*

[a)] Electronic mail: vxg8@psu.edu

### A. Crystal growth and characterization

The $LiOsO_3$ single crystals were grown using solid state reaction under high pressure, as in the previous work by Shi et al[1]. Electron back-scattering diffraction (EBSD) was used to confirm the crystallinity of the samples and orient them. The sample used for SHG polarimetry in this work has its [120] ($X_2$) crystallographic axis oriented along the normal to the probed surface, with the [100] ($X_1$) and [001] ($X_3$) axes along mutually perpendicular directions within the plane. The inverse pole figures obtained from EBSD maps are shown in Fig. S1. The (120) surface was polished using $Ar^+$ ion-milling, with an accelerating voltage of 3 kV run for 30 minutes, after initial hand polishing using calcined alumina polishing paper of roughness 0.3 $\mu m$.

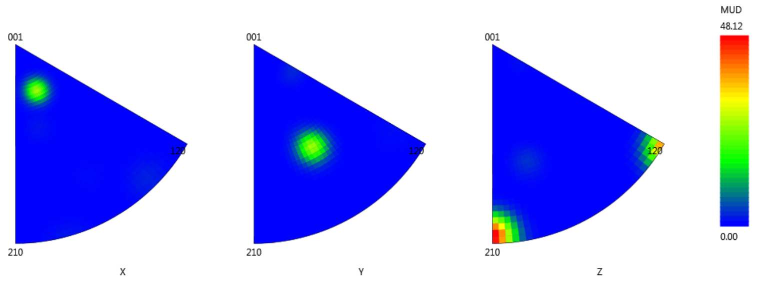


FIG. S1. Inverse pole figures of single crystal $LiOsO_3$ obtained through electron back-scattering diffraction (EBSD).

### B. Spectroscopic ellipsometry

The linear optical susceptibility was measured by spectroscopic ellipsometry carried out using a Woollam M-2000F Focused Beam Spectroscopic Ellipsometer. The measurement was done from 1.2 to 6.2 eV (200 to 1000 nm) using a CCD detector, with the beam incident at an angle of $65.23^o$, and focused onto a spot size of 65 x 20 $\mu m$ on the (120) surface of a $LiOsO_3$ single crystal. The anisotropy in the linear optical properties is obtained by carrying out separate measurements with the plane of incidence parallel to the [001] and [100] directions respectively, in order to simplify the Jones matrix elements[2].

The two sets of data were simultaneously fitted using two sets of Lorentz oscillators $\psi_n = \frac{A_n B_n E_n}{E_n^2 - E^2 - i.E_n B_n}$ (including a constant term $\psi_\infty$), where $A_n$ is the amplitude, $B_n$ is the

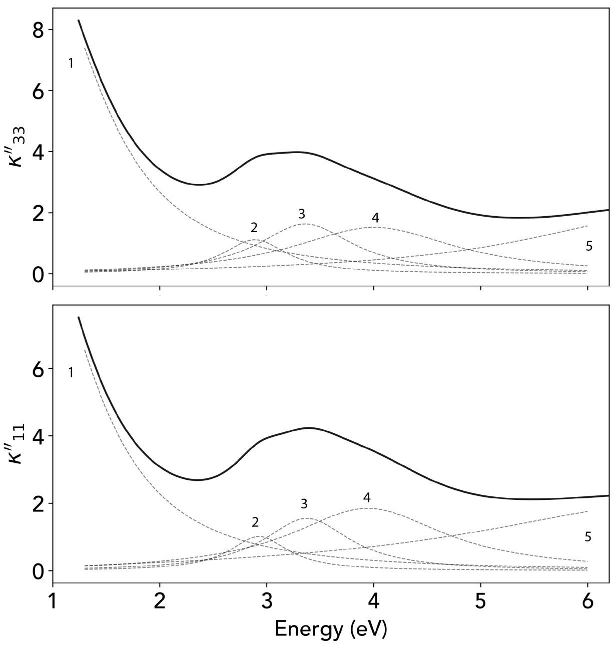


FIG. S2. The imaginary parts of the components of the anisotropic dielectric tensor, $\kappa''_{33}$ and $\kappa''_{11}$, obtained from spectroscopic ellipsometry. The Lorentz oscillators used to fit the data are shown using dotted lines, and with the labels indicating the number n in Table S1.

TABLE S1. The parameters of the Lorentz oscillators used to fit the anisotropic spectroscopic ellipsometry data. The coefficients used to fit $\kappa''_{11}$ are given by $A_n^{11}$, $B_n^{11}$, and $E_n^{11}$, and the coefficients used to fit $\kappa''_{33}$ are given by $A_n^{33}$, $B_n^{33}$, and $E_n^{33}$. The constant terms are $\psi_\infty^{11} = 1.269$, and $\psi_\infty^{33} = 1.796$.

| $n$ | $A_n^{11}$ | $B_n^{11}(eV^{-1})$ | $E_n^{11}(eV)$ | $A_n^{33}$ | $B_n^{33}(eV^{-1})$ | $E_n^{33}(eV)$ |
|---|---|---|---|---|---|---|
| 1 | 9.898 | 1.413 | 0.989 | 9.522 | 1.470 | 1.083 |
| 2 | 1.008 | 0.673 | 2.948 | 1.105 | 0.744 | 2.915 |
| 3 | 1.540 | 0.990 | 3.412 | 1.615 | 1.101 | 3.407 |
| 4 | 1.827 | 1.763 | 4.042 | 1.498 | 1.848 | 4.111 |
| 5 | 1.975 | 4.538 | 7.221 | 1.881 | 3.202 | 6.924 |

FWHM, and $E_n$ is the energy center of the Lorentz oscillator $\psi_n$, to obtain the complex refractive index $\tilde{n} = n + ik$ along the ordinary and extraordinary directions in the crystal. The Bruggeman effective medium approximation was used to characterize surface roughness, consisting of 50 % material and 50 % air. All the data acquisition and analysis was done

using the CompleteEASE software package. The imaginary part of the dielectric function, and the associated Lorentz oscillators are shown in Fig. S2. The values of the parameters of the Lorentz oscillators are shown in Table S1.

### C. SHG polarimetry

The SHG polarimetry measurements described in the main text were done at normal incidence. Since $d_{22}$ was not experimentally accessible in this geometry, an additional polar plot was measured at a $45^o$ angle of incidence to the (120) surface. The sample was aligned so that [120] and [001] were in the plane of incidence. The polar plot was obtained by measuring the second harmonic intensity as a function of polarization direction of the fundamental. The theoretical expression for the reflected second harmonic intensity $I^{2\omega}$ was derived using the method in the paper by Bloembergen and Pershan[3].

$$
\begin{aligned}
E_S^{2\omega}(\phi) &= cos^2(\phi)(\frac{1}{2}B_3 t_p^2 d_{33} cos^2(\theta_t) - B_2 t_p^2 d_{15} sin(2\theta_t) + (B_2 d_{22} + B_3 d_{31}) t_p^2 sin^2(\theta_t)) \\
&\quad + sin^2(\phi)(-B_2 d_{22} + B_3 d_{31}) t_s^2 \\
E_P^{2\omega}(\phi) &= sin(2\phi) B_1 t_p t_s (d_{15} cos(\theta_t) + d_{22} sin(\theta_t)) \\
I^{2\omega} &\propto (E_S^{2\omega})^2 + (E_P^{2\omega})^2
\end{aligned}
\tag{S1}
$$

The constants $t_s$ and $t_p$ are Fresnel coefficients for transmission of s and p components of polarization, $B_i$ (i = 1, 2, 3) are the Bloembergen-Pershan factors relating the second harmonic electric field to the second harmonic polarization along the hexagonal crystallographic directions [100], [120], and [001] respectively, and $\theta_t$ is the angle of transmission of the fundamental beam in the crystal. Plugging in the linear optical constants (see Fig. 1 in main text) and values obtained for $d_{15}$, $d_{31}$, and $d_{33}$ from normal incidence SHG polarimetry (see Table 1 in main text), $d_{22}$ was extracted by fitting to the experimental data.

SHG polarimetry measurements were done as a function of temperature. While the SHG tensor coefficients change in magnitude as in Fig. 2 of the main article, the ratios of the coefficients remain constant as shown in Fig. S4.

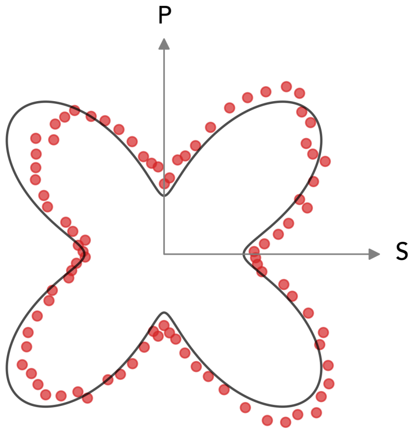


FIG. S3. Polar plot of the SHG intensity as a function of polarization of the fundamental, with an angle of incidence of $45^o$. The solid line is a theory fit to 3m point group symmetry.

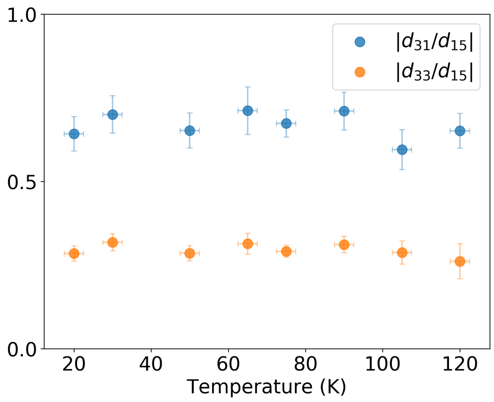


FIG. S4. SHG susceptibility coefficient ratios as a function of temperature.

### D. Bond anisotropy and SHG coefficients in $LiMO_3$ (M = Nb, Ta, Os)

Table II lists the Li-O and M-O bond lengths and the associated bond anisotropy across the family $LiMO_3$ (M = Nb, Ta, Os). The weak coupling mechanism of polar displacements in $LiOsO_3$ results in the smallest $MO_6$ anisotropy. Table III lists the ratios of [001] and [100] projections of the long and short M-O bonds, which is a measure of the $MO_6$ anharmonicity along these two directions. The $MO_6$ anharmonicity along [001] can be related to $d_{33}$, while the anharmonicity along [100] can be related to $d_{22}$ and $d_{31}$. The anharmonicity along [001]

TABLE S2. Li-O and M-O bond lengths in $LiMO_3$ (M = Nb, Ta, Os). The long bonds are denoted by (l) and the short bonds by (s).

| | Li-O (l) | Li-O (s) | Li-O (l)/Li-O (s) | M-O (l) | M-O (s) | M-O (l)/M-O (s) |
|---|---|---|---|---|---|---|
| $LiNbO_3$[a] | 2.239 | 2.068 | 1.083 | 2.112 | 1.889 | 1.118 |
| $LiTaO_3$[b] | 2.293 | 2.076 | 1.038 | 2.073 | 1.891 | 1.096 |
| $LiOsO_3$[c] | 2.312 | 1.929 | 1.199 | 1.960 | 1.930 | 1.016 |

[a] Values at 297 K from reference 4.
[b] Values at 297 K from reference 5.
[c] Values at 20 K from reference 1

TABLE S3. Ratios of the [001] and [100] projections of long and short M-O bonds, and the optical SHG tensor coefficients $d_{ij}$ for $LiMO_3$ (M = Nb, Ta, Os). The long bonds are denoted by (l) and the short bonds by (s).

| | M-O (l)/M-O (s) [001] | M-O (l)/M-O (s) [100] | $\|d_{22}\|$ | $\|d_{31}\|$ | $\|d_{33}\|$ |
|---|---|---|---|---|---|
| $LiNbO_3$[a] | 1.576 | 0.942 | 3.5 (0.8) | 4.6 (0.7) | 32.4 (8.1) |
| $LiTaO_3$[b] | 1.398 | 0.969 | 1.2 (0.1) | 1.0 (0.2) | 15.6 (2.0) |
| $LiOsO_3$[c] | 0.942 | 1.052 | 2.3 (0.2) | 1.9 (0.1) | 0.93 (0.03) |

[a] Values at 297 K from reference 4
[b] Values at 297 K from reference 5
[c] Values at 20 K from reference 1

decreases significantly in $LiOsO_3$, resulting in a suppressed $d_{33}$. The anharmonicity along [100] is relatively uniform, resulting in $d_{22}$ and $d_{31}$ each having the same order of magnitude in all three materials.

## E. Raman spectroscopy

Raman spectroscopy measurements were carried out using a Horiba LabRam confocal microscope. A 532 nm fundamental at a power of 1.5 mW was focused onto the surface of the sample at normal incidence using a 50x objective with a numerical aperture of 0.5. A LN2 cooled InGaAs array detector and a 600 lines/mm grating with a spectral resolution

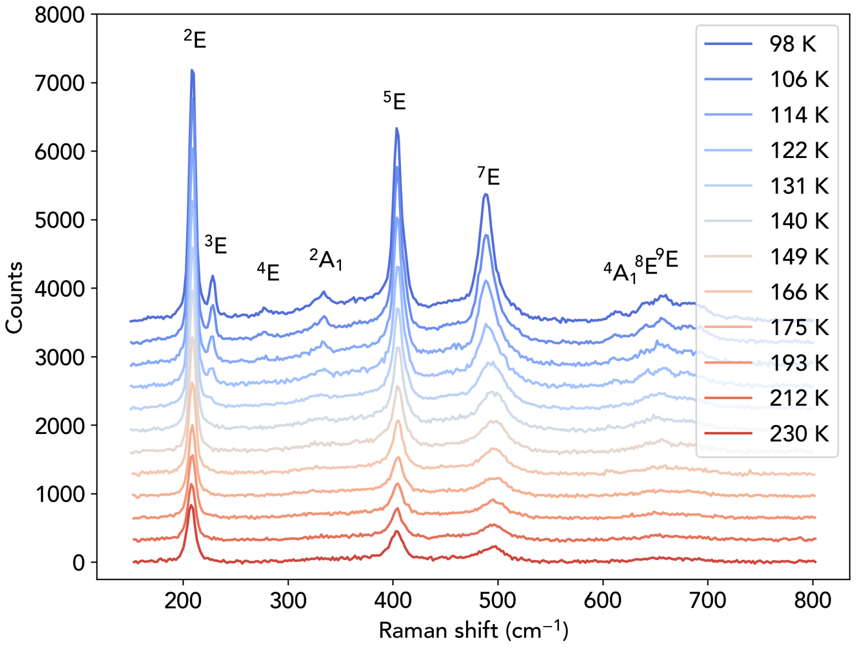


FIG. S5. Raman spectra as a function of temperature, with the peaks labeled as in the work by Jin et al[6].

of 2 $cm^{-1}$ were used to collect the spectra. Low temperature measurements were carried out using a Linkam THMS cryostat. Laser heating was accounted for by calibrating the temperature using the Stokes and anti-Stokes peaks of the Raman phonon mode at 206 $cm^{-1}$, using the below formula -

$$\frac{I_{AS}}{I_S} = \left(\frac{v_l + v_v}{v_l - v_v}\right)^3 exp\left(-\frac{hv_v}{k_B T}\right), \tag{S2}$$

where $I_S$ and $I_{AS}$ are the Stokes and anti-Stokes intensities respectively, $v_l$ and $v_v$ are the frequencies of the laser and considered phonon mode respectively, in units of $s^{-1}$. Since the obtained calibration curve was noisy, the experimentally measured specific heat from reference 1 was used to fit the calibration curve and determine error bars.

A representative set of measured spectra are shown in Fig. S5, with the peaks labeled according to the nomenclature in the work by Jin et al[6].

The peaks were fitted using Lorentzian-Gaussian functions as in the previous work by Jin et al[6], after fitting a second order polynomial to fit and subtract the baseline.

## F. Orienting ferroelastic domains

The orientation of ferroelastic domains was obtained using EBSD. Figure S6 shows an Euler angle map of the striped domains, along with the associated inverse pole figures (IPFs). The black regions in the Euler map correspond to areas where the orientation could not be found by the EBSD fitting, likely due to surface roughness. As the map shows, the stripes have alternating crystallographic orientations. An analysis of the Euler angles shows that these crystallographic orientations are rotated by $90^o$ relative to each other, consistent with the geometry of $109^o/71^o$ domain walls in a trigonal crystal structure. For such a domain structure, the [100] axis must be mutually orthogonal in neighboring domains. This is confirmed by the IPFs. The datapoints on the IPF with higher density correspond to the thick domains, while the datapoints with lower density correspond to the thin domains. The Y IPF shows that the thin domains are oriented with the [100] axis roughly parallel to the sample Y direction, while the Z IPF shows that the thick domains are oriented with the $[110] \equiv [100]$ axis roughly parallel to the sample Z direction.

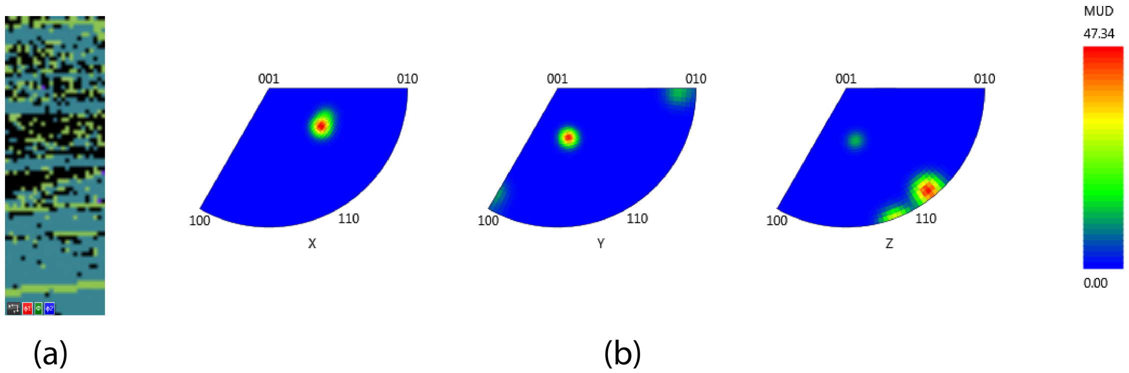


FIG. S6. (a) An Euler angle map of striped ferroelastic domains. (b) The inverse pole figures corresponding to the Euler angle map.

## REFERENCES

[1]Y. Shi, Y. Guo, X. Wang, A. J. Princep, D. Khalyavin, P. Manuel, Y. Michiue, A. Sato, K. Tsuda, S. Yu, M. Arai, Y. Shirako, M. Akaogi, N. Wang, K. Yamaura, and A. T. Boothroyd, Nature Materials **12**, 1024 (2013).

[2]H. Fujiwara, Spectroscopic Ellipsometry: Principles and Applications , 209 (2007).

[3]P. S. Bloembergen, N. and Pershan, Physical Review **128** (1962).

[4]S. Abrahams, J. M. Reddy, and J. Bernstein, Journal of Physics and Chemistry of Solids **27**, 997 (1966).

[5]S. Abrahams and J. Bernstein, Journal of Physics and Chemistry of Solids **28**, 1685 (1967).

[6]F. Jin, A. Zhang, J. Ji, K. Liu, L. Wang, Y. Shi, Y. Tian, X. Ma, and Q. Zhang, Physical Review B **93**, 1 (2016).
